# Supplementary material for: Exact and Approximate Heterogeneous Bayesian Decentralized Data Fusion
Source: arXiv:2101.11116 source file (2024-01-29)
Supplement: Supplementary file 1 [file Appendix_iAS.tex]

The augmented state for a sliding time window from time step $n$ to time step $k$ (denoted by subscript $k:n$) as shown in \cite{chong_comparison_2014} is given by the following equations:\\
\emph{Prediction Step}
\begin{equation}
        X_{k:n|k-1}=\begin{pmatrix}F_{k-1}\chi_{k-1|k-1}+Gu_k \\ X_{k-1:n|k-1}
        \end{pmatrix}
        \label{eq:AS_pred_vec}
\end{equation}
\begin{equation}
       P_{k:n|k-1}=\begin{pmatrix} P_{k|k-1} & \mathbf{F}P_{k-1:n|k-1}  \\
       P_{k-1:n|k-1}\mathbf{F}^T  & P_{k-1:n|k-1}
        \end{pmatrix},
        \label{eq:AS_pred_mat}
\end{equation}
where $\mathbf{F}=\big[F_{k-1} \ \ 0_{m \times m(k-n-2)} \big ]$ and $m$ is the size of the (not augmented) state vector.\\
\emph{Update Step}\\
The measurement update in information space is as follows:
\begin{equation}
       P_{k:n|k}^{-1}= P_{k:n|k-1}^{-1}+J_kI_kJ_k^T
       \label{eq:AS_upd_mat}
\end{equation}
\begin{equation}
        P_{k:n|k}^{-1}X_{k:n|k}= P_{k:n|k-1}^{-1}X_{k:n|k-1}+J_ki_k,
        \label{eq:AS_upd_vec}
\end{equation}
where $J_k=\big[I_m \ \ 0_{m \times m(k-n-1)} \big ]^T$, $i_k=H_k^TR_k^{-1}z_k$ and $I_k=H_k^TR_k^{-1}H_k$.

%\subsection{Information Augmented State (iAS) Filter}
%\label{ssec:iASF}
Since the algorithms developed in this paper work in log space, it is advantageous to work with an information filter, which is based on the log-likelihood of the Gaussian distribution. Thus, a transformation of the prediction step given in (\ref{eq:AS_pred_vec})-(\ref{eq:AS_pred_mat}) from state space to the Gaussian information space is needed. 

First, define $P_{k:n|k-1}^{-1}$ to be the augmented predicted information matrix:
\begin{equation}
    \begin{split}
       P_{k:n|k-1}^{-1}
        &=\begin{pmatrix} V_{11}  &  V_{12} \\ V_{21}  & V_{22} \end{pmatrix},
    \end{split}
        \label{eq:iAS_pred_mat}
\end{equation}
where from the matrix inversion lemma:
\begin{equation}
    \begin{split}
        V_{11} &= (P_{k|k-1}-\mathbf{F}P_{k-1:n|k-1}P_{k-1:n|k-1}^{-1}P_{k-1:n|k-1}\mathbf{F}^T)^{-1}\\
        &=(P_{k|k-1}-\mathbf{F}P_{k-1:n|k-1}\mathbf{F}^T)^{-1}.
    \end{split}
    \label{eq:V11a}
\end{equation}
The expression $\mathbf{F}P_{k-1:n|k-1}\mathbf{F}^T$ has the dimension $m\times m$. From the definition of $\mathbf{F}$ above (\ref{eq:V11a}) can be simplified by noticing that 
$\mathbf{F}P_{k-1:n|k-1}\mathbf{F}^T = F_{k-1}P_{k-1|k-1}F_{k-1}^T$, i.e. it depends only on the previous time step and not the full time history. Eq. (\ref{eq:V11a}) is thus:
\begin{equation}
        V_{11} = (P_{k|k-1}- F_{k-1}P_{k-1|k-1}F_{k-1}^T)^{-1}.
    \label{eq:V11b}
\end{equation}
Here $P_{k|k-1}^{-1}$ is the predicted information matrix at time step $k$, given in the literature by: $P_{k|k-1}^{-1}=(F_{k-1}P_{k-1|k-1}F_{k-1}^T+Q)^{-1}$, where $Q$ is the process noise covariance. 
%where $A_{k-1}^{-1}=(F_{k-1}P_{k-1|k-1}F_{k-1}^T)$.
Taking the inverse and plugging in $P_{k|k-1}$, (\ref{eq:V11b}) can be simplified to: 
\begin{equation}
    V_{11}=Q^{-1}.
    \label{eq:V11_simple}
\end{equation}
Applying the matrix inversion lemma again the expressions for other terms are: 
\begin{equation}
        V_{12} =V_{21}^T = -V_{11}\mathbf{F}P_{k-1:n|k-1}P_{k-1:n|k-1}^{-1}
        =-V_{11}\mathbf{F},
    \label{eq:V12}
\end{equation}
\begin{equation}
    \begin{split}
        V_{22}
        =P_{k-1:n|k-1}^{-1}+\mathbf{F}^TV_{11}\mathbf{F}.
    \end{split}
    \label{eq:V22}
\end{equation}
The predicted information matrix is then given by: 
\begin{equation}
    \begin{split}
       P_{k:n|k-1}^{-1}=
       \begin{pmatrix} Q^{-1} & -Q^{-1}\Gamma^T\mathbf{F}  \\
       -\mathbf{F}^T\Gamma Q^{-1}  & P_{k-1:n|k-1}^{-1}+\mathbf{F}^T\Gamma Q^{-1}\Gamma^T\mathbf{F}
        \end{pmatrix}\\
    \end{split}
        \label{eq:iAS_pred_matFinal}
\end{equation}
\begin{comment}

\begin{equation}
    \begin{split}
       P_{k:n|k-1}^{-1}=
       \begin{pmatrix} Q^{-1} & -Q^{-1}\mathbf{F}  \\
       -\mathbf{F}^TQ^{-1}  & P_{k-1:n|k-1}^{-1}+\mathbf{F}^TQ^{-1}\mathbf{F}
        \end{pmatrix}\\
    \end{split}
        \label{eq:iAS_pred_matFinal}
\end{equation}
\end{comment}
and the predicted information vector can now be derived:
\begin{comment}
\begin{equation}
    \begin{split}
       &P_{k:n|k-1}^{-1}X_{k:n|k-1}=\begin{pmatrix} V_{11}  &  V_{12} \\ V_{21}  & V_{22} \end{pmatrix}\begin{pmatrix}F_{k-1}\xi_{k-1|k-1}+Gu_k \\ X_{k-1:n|k-1}\end{pmatrix}\\
       &=\begin{pmatrix}Q^{-1}Gu_k \\ 
       P_{k-1:n|k-1}^{-1}X_{k-1:n|k-1}-\mathbf{F}^TQ^{-1}Gu_k\end{pmatrix}
    \end{split}
    \label{eq:iAS_pred_vecFinal}
\end{equation}
\end{comment}
\begin{equation}
    \begin{split}
       P_{k:n|k-1}^{-1}&X_{k:n|k-1}=\\
       &\begin{pmatrix}Q^{-1}Gu_k \\ 
       P_{k-1:n|k-1}^{-1}X_{k-1:n|k-1}-\mathbf{F}^T\Gamma Q^{-1}Gu_k\end{pmatrix}.
    \end{split}
    \label{eq:iAS_pred_vecFinal}
\end{equation}
\begin{comment}

\begin{equation}
    \begin{split}
       P_{k:n|k-1}^{-1}&X_{k:n|k-1}=\\
       &\begin{pmatrix}Q^{-1}Gu_k \\ 
       P_{k-1:n|k-1}^{-1}X_{k-1:n|k-1}-\mathbf{F}^TQ^{-1}Gu_k\end{pmatrix}.
    \end{split}
    \label{eq:iAS_pred_vecFinal}
\end{equation}
\end{comment}
