# Supplementary material for: Exact and Approximate Heterogeneous Bayesian Decentralized Data Fusion
Source: arXiv:2101.11116 source file (2024-01-29)
Supplement: Supplementary file 2 [file AppendixArchive.tex]

Here I am starting to summarize the advancements from the MFI 2020 paper.\\
The main subjects are as follows:
\begin{enumerate}
    \item Summary of the augmented state filter (ASF) - \ref{ssec:ASF}
    \item Derivation of the information form AS-filter (iASF) - \ref{ssec:iASF}
    \item Implementation of sliding window, including assimilation of the full state before fusion + Saving only position and velocity states in time - \ref{ssec:slidingWin}
    \item Block-tridiagonal matrix inversion - \ref{ssec:matrixInversion}
    \item Probabilistic analysis
\end{enumerate}

\subsection{Augmented State (AS) Filter}
\label{ssec:ASF}
The augmented state filter as shown in ref.\cite{chong_comparison_2014} is given by  the following equations:\\
\emph{Prediction}
\begin{equation}
        X_{k:n|k-1}=\begin{pmatrix}F_{k-1}\chi_{k-1|k-1}+Gu_k \\ X_{k-1:n|k-1}
        \end{pmatrix}
        \label{eq:AS_pred_vec}
\end{equation}
\begin{equation}
       P_{k:n|k-1}=\begin{pmatrix} P_{k|k-1} & \mathbf{F}P_{k-1:n|k-1}  \\
       P_{k-1:n|k-1}\mathbf{F}^T  & P_{k-1:n|k-1}
        \end{pmatrix}
        \label{eq:AS_pred_mat}
\end{equation}
here $\mathbf{F}=\big[F_{k-1} \ \ 0_{m \times m(k-n-2)} \big ]$ and $m$ is the size of the (not augmented) state vector.
\emph{Update}
The measurement update is done in information space as follows:
\begin{equation}
       P_{k:n|k}^{-1}= P_{k:n|k-1}^{-1}+J_kI_kJ_k^T
       \label{eq:AS_upd_mat}
\end{equation}
\begin{equation}
        P_{k:n|k}^{-1}X_{k:n|k}= P_{k:n|k-1}^{-1}X_{k:n|k-1}+J_ki_k
        \label{eq:AS_upd_vec}
\end{equation}
where $J_k=\big[I_m \ \ 0_{m \times m(k-n-1)} \big ]^T$, $i_k=H_k^TR_k^{-1}z_k$ and $I_k=H_k^TR_k^{-1}H_k$.


\subsection{Information Augmented State (iAS) Filter}
\label{ssec:iASF}
Since the information fusion algorithms work in information space, it might be advantageous to work with an information filter. Thus we need to formulate the prediction step given in equations (\ref{eq:AS_pred_vec})-(\ref{eq:AS_pred_mat}). \\ 
First, define $P_{k:n|k-1}^{-1}$ to be the augmented predicted information matrix:
\begin{equation}
    \begin{split}
       P_{k:n|k-1}^{-1}&=\begin{pmatrix} P_{k|k-1} & \mathbf{F}P_{k-1:n|k-1}  \\
       P_{k-1:n|k-1}\mathbf{F}^T  & P_{k-1:n|k-1}
        \end{pmatrix}^{-1}\\
        &=\begin{pmatrix} V_{11}  &  V_{12} \\ V_{21}  & V_{22} \end{pmatrix}
    \end{split}
        \label{eq:iAS_pred_mat}
\end{equation}

\begin{equation}
    \begin{split}
        V_{11} &= (P_{k|k-1}-\mathbf{F}P_{k-1:n|k-1}P_{k-1:n|k-1}^{-1}P_{k-1:n|k-1}\mathbf{F}^T)^{-1}\\
        &=(P_{k|k-1}-\mathbf{F}P_{k-1:n|k-1}\mathbf{F}^T)^{-1}
    \end{split}
    \label{eq:V11a}
\end{equation}
We can observe that the expression $\mathbf{F}P_{k-1:n|k-1}\mathbf{F}^T$ has the dimension $m\times m$ and that because of how we define $\mathbf{F}$, it can be written as $\mathbf{F}P_{k-1:n|k-1}\mathbf{F}^T = F_{k-1}P_{k-1|k-1}F_{k-1}^T$, i.e. it depends only on the previous time step and not the full time history. Eq. (\ref{eq:V11a}) is thus:
\begin{equation}
        V_{11} = (P_{k|k-1}- F_{k-1}P_{k-1|k-1}F_{k-1}^T)^{-1}.
    \label{eq:V11b}
\end{equation}

\begin{comment}
Using the matrix inversion Lemma a few times, the final expression for $V_{11}$ is:
\begin{equation}
        V_{11} = P_{k|k-1}^{-1}\bigg (I+(A_{k-1}-P_{k|k-1}^{-1})^{-1}P_{k|k-1}^{-1}\bigg),
    \label{eq:V11Final}
\end{equation}
\end{comment}
where $A_{k-1}^{-1}=(F_{k-1}P_{k-1|k-1}F_{k-1}^T)$ and $P_{k|k-1}^{-1}$ is the predicted information matrix at time step $k$, given in the literature by: $P_{k|k-1}^{-1}=(A_{k-1}^{-1}+Q)^{-1}$. Taking the inverse, plugging in the definition of $A_{k-1}^{-1}$, eq. (\ref{eq:V11b}) can be simplified to: 
\begin{equation}
    V_{11}=Q^{-1}
    \label{eq:V11_simple}
\end{equation}


The cross-covariance terms $V_{12}=V_{21}^T$ are given by:
\begin{equation}
        V_{12} =V_{21}^T = -V_{11}\mathbf{F}P_{k-1:n|k-1}P_{k-1:n|k-1}^{-1}
        =-V_{11}\mathbf{F}.
    \label{eq:V12}
\end{equation}
The last expression is rather easy to find and given by:
\begin{equation}
    \begin{split}
        V&_{22} = P_{k-1:n|k-1}^{-1}\\
        &+P_{k-1:n|k-1}^{-1}P_{k-1:n|k-1}\mathbf{F}^TV_{11}\mathbf{F}P_{k-1:n|k-1}P_{k-1:n|k-1}^{-1}\\
        &=P_{k-1:n|k-1}^{-1}+\mathbf{F}^TV_{11}\mathbf{F}.
    \end{split}
    \label{eq:V22}
\end{equation}
The predicted information matrix is then given by: 
\begin{equation}
    \begin{split}
       P_{k:n|k-1}^{-1}=
       \begin{pmatrix} Q^{-1} & -Q^{-1}\mathbf{F}  \\
       -\mathbf{F}^TQ^{-1}  & P_{k-1:n|k-1}^{-1}+\mathbf{F}^TQ^{-1}\mathbf{F}
        \end{pmatrix}\\
    \end{split}
        \label{eq:iAS_pred_matFinal}
\end{equation}
\begin{comment}
\begin{figure*}[tb]
\begin{equation}
    \begin{split}
       P_{k:n|k-1}^{-1}=
       \begin{pmatrix} P_{k|k-1}^{-1} (I+(A_{k-1}-P_{k|k-1}^{-1})^{-1}P_{k|k-1}^{-1}) & -V_{11}\mathbf{F}  \\
       -\mathbf{F}^TV_{11}  & P_{k-1:n|k-1}^{-1}+\mathbf{F}^TV_{11}\mathbf{F}
        \end{pmatrix}\\
    \end{split}
        \label{eq:iAS_pred_matFinal}
\end{equation}
\end{figure*}
\end{comment}
The predicted information vector can now be derived:
\begin{equation}
    \begin{split}
       P_{k:n|k-1}^{-1}&X_{k:n|k-1}=\begin{pmatrix} V_{11}  &  V_{12} \\ V_{21}  & V_{22} \end{pmatrix}\begin{pmatrix}F_{k-1}\xi_{k-1|k-1}+Gu_k \\ X_{k-1:n|k-1}\end{pmatrix}\\
       &=\begin{pmatrix}Q^{-1}Gu_k \\ 
       P_{k-1:n|k-1}^{-1}X_{k-1:n|k-1}-\mathbf{F}^TQ^{-1}Gu_k\end{pmatrix}
    \end{split}
    \label{eq:iAS_pred_vecFinal}
\end{equation}
It is important to mention that from the definition of $\mathbf{F}$ it results that the structure of the updated information matrix $P_{k:n|k-1}^{-1}$ is block-tridiagonal, this is also demonstrated in a similar but not equivalent filter, named accumulated state density given in \cite{koch_accumulated_2011}.

\subsection{Sliding Window}
\label{ssec:slidingWin}

Keeping the full time history from $t=0$ until time step $k$ will lead to a very large state vector and covariance matrix ($mk\times mk$). 
A solution to this problem is keeping only a part of the augmented state in a certain sliding window ($k:n$), this is done by marginalizing out past state (of time steps before $n$). However, in our problem, this will result coupling of the local (conditionally independent) states $s_i$ and $s_j$. 
We use the formulation given in eq. (\ref{eq:localInfFusion}) to suggest a method to incorporate the sliding window mechanism, while allowing the reconstruction of the full augmented state to regain conditional independence.

\begin{equation}
    \begin{split}
        \Lambda_{k:n-1|k}&=\begin{pmatrix} \Lambda_{k:n,k:n}  & \Lambda_{k:n,n-1} \\
        \Lambda_{n-1,k:n} & \Lambda_{n-1,n-1}\end{pmatrix}\\
        &=\begin{pmatrix} \bar{\Lambda}_{k:n,k:n}  & 0 \\
        0 &0\end{pmatrix}\\
        &+\begin{pmatrix} \Lambda_{k:n,n-1}\Lambda_{n-1,n-1}^{-1}\Lambda_{n-1,k:n}  & \Lambda_{k:n,n-1} \\
        \Lambda_{n-1,k:n} & \Lambda_{n-1,n-1}\end{pmatrix}
    \end{split}
    \label{eq:slideWin}
\end{equation}
here we dropped the conditioning on the $k-th$ measurement for abbreviation. We note that $\Lambda$ here is the information matrix, i.e. $\Lambda_{k:n-1|k}=P^{-1}_{k:n-1|k}$ as given in eq. (\ref{eq:AS_upd_mat}). 
A similar formulation for the information vector is straight forward. \\
In the above equation the first matrix is the marginal information over the states in the time window $k:n$, given by $\bar{\Lambda}_{k:n,k:n}$, while the matrix $\Lambda_{k:n-1|k}$ is the information over the time window $k:n-1$, after the measurement update at time step $k$. The last matrix holds information regrading the past state and allows reconstruction of the full matrix $\Lambda_{k:n-1|k}$. In order to reconstruct the full time history this information has to be stored in each time step. Then a recursive assimilation can be implemented to build the full information matrix $\Lambda_{k:0|k}$ and regain conditional independence (after inversion). This will be explained next.\\
For simplicity assume $k=2,n=1$, i.e. a sliding window of 2 time steps. Eq. (\ref{eq:slideWin}) is then:
\begin{equation}
    \begin{split}
        &\Lambda_{2:0|2}=\begin{pmatrix} \Lambda_{2:1,2:1}  & \Lambda_{2:1,0} \\
        \Lambda_{0,2:1} & \Lambda_{0,0}\end{pmatrix}\\
        &=\begin{pmatrix} \bar{\Lambda}_{2:1,2:1}  & 0 \\
        0 &0\end{pmatrix}+\begin{pmatrix} \Lambda_{2:1,0}\Lambda_{0,0}^{-1}\Lambda_{0,2:1}  & \Lambda_{2:1,0} \\
        \Lambda_{0,2:1} & \Lambda_{0,0}\end{pmatrix}
    \end{split}
    \label{eq:slideWin_2_0}
\end{equation}
wheres as we mentioned before, the last matrix has to be stored in order to reconstruct the full information matrix later. \\
After marginalizing, we are left with the marginal information matrix $\Lambda_{2:1|2}=\bar{\Lambda}_{2:1,2:1}$. Completing a prediction-update cycle, the new augmented information matrix is now $\Lambda_{3:1|3}$, given by:
\begin{equation}
    \begin{split}
        \Lambda_{3:1|3}=\begin{pmatrix} \Lambda_{3,3}  & \Lambda_{3,2:1} \\
        \Lambda_{2:1,3} & \Lambda_{2:1,2:1}\end{pmatrix}\\
    \end{split}
    \label{eq:slideWin_3_1}
\end{equation}
We are interested now in assimilating the full information matrix $\Lambda_{3:0|3}$.
\begin{equation}
    \begin{split}
        \Lambda_{3:0|3}=\begin{pmatrix} \Lambda_{3,3}  & \Lambda_{3,2:1} & \Lambda_{3,0} \\ \Lambda_{2:1,3} & \Lambda_{2:1,2:1} & \Lambda_{2:1,0} \\
        \Lambda_{0,3} & \Lambda_{0,2:1} & \Lambda_{0,0}
        \end{pmatrix}\\
    \end{split}
    \label{eq:slideWin_3_0}
\end{equation}
As mentioned before, the structure of this matrix is block-tridiagonal, thus $\Lambda_{0,3} = \Lambda_{3,0}=\pmb{0}$ (this also implies that $\Lambda_{1,3} = \Lambda_{3,1}=\pmb{0}$). Remember that in eq. (\ref{eq:slideWin_3_1}), $\Lambda_{2:1,2:1}$ is an updated version of the marginal information given in eq. (\ref{eq:slideWin_2_0}), so by adding zeros in the correct dimension and summing eq. (\ref{eq:slideWin_2_0}) and (\ref{eq:slideWin_3_1}) we get:

\begin{equation}
    \begin{split}
        \Lambda_{3:0|3}=\begin{pmatrix} \Lambda_{3,3}  & \Lambda_{3,2:1} & \pmb{0} \\ \Lambda_{2:1,3} & \bar{\Lambda}_{2:1,2:1}+\Lambda_{2:1,0}\Lambda_{0,0}^{-1}\Lambda_{0,2:1} & \Lambda_{2:1,0} \\
        \pmb{0} & \Lambda_{0,2:1} & \Lambda_{0,0}
        \end{pmatrix}\\
    \end{split}
    \label{eq:slideWin_3_0_final}
\end{equation}
which is the full information matrix that we where looking for.\\
Figure \ref{fig:matrixAssimilation} visualizes the marginalization and assimilation process, where each square is a block matrix corresponding to the information state vector at time step $k$, off-diagonal squares relate to the cross blocks in time steps $k$ and $n$, $k\neq n$. The dark square mark blocks that are without change relative to a full filtering, without a sliding window. In (a) the separation of the full information matrix $\Lambda_{2:0|2}$ (eq. (\ref{eq:slideWin_2_0})) into two matrices: the marginal information matrix $\bar{\Lambda}_{2:1|2}$ and information matrix that relates to the conditional information $\log p(X_{0}|X_{2:1})$.
In (b) it is shown that most blocks in the sub-matrix $\Lambda_{2:1,0}\Lambda_{0,0}^{-1}\Lambda_{0,2:1}$ are zero-blocks, i.e. this sub-matrix only hold information related to time step 1. From this we can conclude that most blocks in the marginal matrix $\bar{\Lambda}_{2:1|2}$, as seen in the first part in (c). The second part in (c) show a full cycle of prediction-update as given by eq. (\ref{eq:iAS_pred_matFinal}) and (\ref{eq:AS_upd_mat}) preformed over the marginalized distribution $\bar{\Lambda}_{2:1,2:1}$. As shown in the equations above, this update is only a function of the previous time step, that has two results: 1. there is no affect to the marginalization in step (a) on the outcome of these steps. 2. there is no contribution, nor from the prediction step nor from the update step to the right lower corner block.
In (d) we see the assimilation process - summing the results of (c) and (a)-(b) we can see the we can reconstruct the full information matrix $\Lambda_{3:0|3}$ without losing any information in the process.

\begin{figure*}[bt]
	\centering
	\includegraphics[width=0.9\textwidth]{Figures/matrix_visualization.png}
	\caption{ } 
	\label{fig:matrixAssimilation}
	\vspace{-0.25in}
\end{figure*}

While this formulation enables a reduction in computation complexity in the filter, it still requires the inversion of almost the full information matrix in the fusion algorithm, when all time history has to be conditioned to regain conditional independence.

% Maybe I need to mention here a Markov property?

% Also, maybe needs a citation like Kavcic for more justification

\subsection{Block-Tridiagonal Matrix Inversion}
\label{ssec:matrixInversion}

\subsection{Probabilistic Analysis}
\label{probAnalysis}

Remember the basic factorized fusion rule that we are trying to solve, using eq. (\ref{eq:exactFusion_3states}):
\begin{equation}
    \begin{split}
     &p_f(\chi|Z_i\cup Z_j)=\frac{1}{C}\cdot\frac{p_i(x|Z_i)p_j(x|Z_j)}{p_c(x|Z_i\cap Z_j)}\cdot \\&\frac{p_i(s_i|x,Z_i)p_j(s_i|x,Z_j)}{p_c(s_i|x,Z_i\cap Z_j)}\cdot\frac{p_i(s_j|x,s_i,Z_i)p_j(s_j|x,s_i,Z_j)}{p_c(s_j|x,s_i,Z_i\cap Z_j)}
    \end{split}
    %\label{eq:exactFusion_3states}
\end{equation}
In a dynamic system, in order to apply conditional independence, we need to condition on all past state. For this reason, the distribution in the above equation is the full posterior augmented distribution, $p(x_{k:0},s_{i,k:0},s_{j,k:0}|Z_k)$, where $Z_k$ is all the data available at time $k$.\\

\emph{Sliding window:}\\
Factorizing the full distribution gives the following:
\begin{equation}
    \begin{split}
        &p(x_{k:0},s_{i,k:0},s_{j,k:0}|Z_k)=p(x_{k:n},s_{i,k:n},s_{j,k:n}|Z_k)\\ 
        &\cdot p(x_{n-1:0},s_{i,n-1:0},s_{j,n-1:0}|x_{k:n},s_{i,k:n},s_{j,k:n},Z_k).
    \end{split}
    \label{factorizedAug}
\end{equation}
It is important to note here that in the literature, both the augmented and accumulated state filters marginalize out past states in their sliding window, thus losing part of the information available in the full distribution. As we demonstrated in \ref{ssec:slidingWin}, by storing the conditional distribution we are able to reconstruct the full augmented distribution.
Note, that for conditional independence, only the target state time history is required, thus the distribution that we are interested can be reduced to $p(x_{k:0},s_{i,k:n},s_{j,k:n}|Z_k)$, or if we further assume that the ownship states are static, the distribution is  $p(x_{k:0},s_{i},s_{j}|Z_k)$:
\begin{equation}
    \begin{split}
        &p(x_{k:0},s_{i},s_{j}|Z_k)=\\&p(x_{k:n},s_{i},s_{j}|Z_k) 
        \cdot p(x_{n-1:0}|x_{k:n},s_{i},s_{j},Z_k)
    \end{split}
    \label{eq:factorizedAugReduced}
\end{equation}
where the first distribution on the RHS is the sliding window marginal distribution, and the second is the conditional past target states to be stored. \\
Since in practice, marginalizing and conditioning on the sliding window is done recursively, it is of interest to look closer at  $p(x_{n-1:0}|x_{k:n},s_{i},s_{j},Z_k)$. Assume $m=k-n$ is the window size, then at time step $m+1$ we marginalize out $x_0$:
\begin{equation}
    \begin{split}
        &p(x_{m+1:0},s_{i},s_{j}|Z_{m+1})=\\&p(x_{m+1:1},s_{i},s_{j}|Z_{m+1})\cdot p(x_{0}|x_{m+1:1},s_{i},s_{j},Z_{m+1})
    \end{split}
    %\label{}
\end{equation}
In the following time steps the conditional distributions would be:
$p(x_{1}|x_{m+2:2},s_{i},s_{j},Z_{m+2})$, $p(x_{2}|x_{m+3:3},s_{i},s_{j},Z_{m+3})$ ,..., $p(x_{n-1}|x_{k:n},s_{i},s_{j},Z_{k})$, but from the law of total probability we know that: 
\begin{equation}
    \begin{split}
    \prod_{l=n}^{1}p(x_{l-1}|x_{m+l:l},s_{i},s_{j},Z_{m+l})=p(x_{n-1:0}|x_{k:n},s_{i},s_{j},Z_{k})
    \end{split}
    %\label{}
\end{equation}
\od{here we used the graph in fig. \ref{fig:GraphModel}(b) for the following Markovian assumption: $x_{l-2}\perp x_{m+l:l},Z_{m+l:l} | x_{l-1},s_i,s_j,Z_{l-1}$. Note that here we use $Z_k$ and not $[y_k, m_k]$, this is to account for information from other agents in the network.}\\
Plugin in to eq. (\ref{eq:factorizedAugReduced}), the required augmented distribution is given by:
\begin{equation}
    \begin{split}
        &p(x_{k:0},s_{i},s_{j}|Z_k)=\\&p(x_{k:n},s_{i},s_{j}|Z_k) 
        \cdot \prod_{l=n}^{1}p(x_{l-1}|x_{m+l:l},s_{i},s_{j},Z_{m+l})
    \end{split}
    \label{eq:factorizedAugReduced_2}
\end{equation}
where $p(x_{l-1}|x_{m+l:l},s_{i},s_{j},Z_{m+l})$ for $l=1,..., n$ is generally low-dimensional, and is proportional to the sliding window size.\\
\od{If I want to get rid of the $Z_k$ from here on, I probably need to justify here.}
For heterogeneous fusion we are interested in the distribution $p(s_{i},s_{j}|x_{k:0})$, so the question is how can we efficiently update this distribution from eq. (\ref{eq:factorizedAugReduced_2}).
Marginalizing $x_{k:n}$ and taking out $l=n$ from the multiplier in eq. (\ref{eq:factorizedAugReduced_2}) we get:
\begin{equation}
    \begin{split}
        &p(x_{k:0},s_{i},s_{j})=p(x_{k:n})\cdot p(s_{i},s_{j}|x_{k:n}) \\
        &\cdot p(x_{n-1}|x_{k:n},s_{i},s_{j}) \cdot \prod_{l=n-1}^{1}p(x_{l-1}|x_{m+l:l},s_{i},s_{j})
    \end{split}
    \label{eq:factorizedAugReduced_3}
\end{equation}
but,
\begin{equation}
    \begin{split}
        p(s_{i},s_{j}|x_{k:n})&\cdot p(x_{n-1}|x_{k:n},s_{i},s_{j})
        = p(s_{i},s_{j},x_{n-1}|x_{k:n})\\
        &= p(s_{i},s_{j}|x_{k:n-1})\cdot p(x_{n-1}|x_{k:n}).
    \end{split}
    \label{eq:factorizedAugReduced_4}
\end{equation}
Plugin back into eq. (\ref{eq:factorizedAugReduced_3} and taking out $l=n-1$:
\begin{equation}
    \begin{split}
        &p(x_{k:0},s_{i},s_{j})=p(x_{k:n})\cdot p(x_{n-1}|x_{k:n})\cdot p(s_{i},s_{j}|x_{k:n-1}) \\
        &\cdot p(x_{n-2}|x_{k-1:n-1},s_{i},s_{j}) \cdot \prod_{l=n-2}^{1}p(x_{l-1}|x_{m+l:l},s_{i},s_{j}).
    \end{split}
    \label{eq:factorizedAugReduced_5}
\end{equation}
Now, using Markovian assumption, $p(x_{n-2}|x_{k-1:n-1},s_{i},s_{j})=p(x_{n-2}|x_{k:n-1},s_{i},s_{j})$. This allows us to use the same update as in (\ref{eq:factorizedAugReduced_4}):
\begin{equation}
    \begin{split}
        p(s_{i},s_{j}|x_{k:n-1})&\cdot p(x_{n-2}|x_{k-1:n},s_{i},s_{j})\\
        &= p(s_{i},s_{j},x_{n-2}|x_{k:n-1})\\
        &= p(s_{i},s_{j}|x_{k:n-2})\cdot p(x_{n-2}|x_{k:n-1})\\
        &= p(s_{i},s_{j}|x_{k:n-2})\cdot p(x_{n-2}|x_{k-1:n-1}).
    \end{split}
    \label{eq:factorizedAugReduced_6}
\end{equation}
We can thus recursively update the conditional distribution over the ownship states and re-write eq. (\ref{eq:factorizedAugReduced_2}):
\begin{equation}
    \begin{split}
        p(x_{k:0},s_{i},s_{j})=p(x_{k:n})\cdot p(s_{i},s_{j}|x_{k:0}) 
        \cdot \prod_{l=n}^{1}p(x_{l-1}|x_{m+l:l}).
    \end{split}
    \label{eq:factorizedAugReduced_7}
\end{equation}
To get an expression for $p(s_{i},s_{j}|x_{k:0})$ we take the natural logarithm and subtract eq. (\ref{eq:factorizedAugReduced_7}) from (\ref{eq:factorizedAugReduced_3}):  
\begin{equation}
    \begin{split}
        &\log p(s_{i},s_{j}|x_{k:0})= \log p(s_{i},s_{j}|x_{k:n})\\
        &+\sum_{l=n}^{1}\bigg ( \log p(x_{l-1}|x_{m+l:l},s_{i},s_{j})-\log p(x_{l-1}|x_{m+l:l}) \bigg ).
    \end{split}
    \label{eq:ownship_Update}
\end{equation}
It is important to note that while it is not explicitly shown in the above equation $p(x_{l-1}|x_{m+l:l})$ is a retrodicted marginal target distribution, after updating the current ownship states as shown in eq. (\ref{eq:factorizedAugReduced_4}), i.e. given information up-to and including time step $k$. On the other hand $p(x_{l-1}|x_{m+l:l},s_{i},s_{j})$ is the distribution up-to and including time step $m+l$.\\

\emph{Fusion update:}\\
We now have $p(s_{i},s_{j}|x_{k:0})$, and remember that from conditional independence $p(s_{i},s_{j}|x_{k:0})=p(s_{i}|x_{k:0})\cdot p(s_{j}|x_{k:0})$.\\
Without loss of generality, assume that in fusion we are updating only $p(x_{k:n})$ (and not $p(x_{k:0})$), then:
\begin{equation}
    \begin{split}
        &p_{i,f}(x_{k:0},s_{i},s_{j})=\\
        &=p_{f}(x_{k:n})\cdot p_i(s_{i}|x_{k:0})\cdot p_j(s_{j}|x_{k:0})
        \cdot \prod_{l=n}^{1}p_i(x_{l-1}|x_{m+l:l})\\
        &=p_{f}(x_{k:n})\cdot p_f(s_{i},s_{j}|x_{k:0})
        \cdot \prod_{l=n}^{1}p_i(x_{l-1}|x_{m+l:l}),
    \end{split}
    \label{eq:fusedFactorizedAugReduced}
\end{equation}
where $p_i(\ )$, $p_{f}(\ )$ and $p_{i,f}(\ )$ represent local, fused and local-fused distributions, respectively, and by 'fused' we mean this distributions are identical between the two agents \emph{i} and \emph{j}, as opposed to local-fused, which mean that the distributions will be different between the agents - heterogeneous.
We can now recursively update the distributions $p_i(x_{l-1}|x_{m+l:l})$, where $l=1,..., n$, based on the fused distribution $p_{f}(x_{k:n})$:
\begin{equation}
    \begin{split}
        &p_{i,f}(x_{k:0},s_{i},s_{j})=\\
        &=p_{f}(x_{k:n})\cdot p_f(s_{i},s_{j}|x_{k:0})
        \cdot \prod_{l=n}^{1}p_{i,f}(x_{l-1}|x_{m+l:l}).
    \end{split}
    \label{eq:fusedFactorizedAugReduced_2}
\end{equation}
The last step can be thought of as the inverse of eq. (\ref{eq:factorizedAugReduced_4}), where now we are recursively updating the ownship states distribution and marginalizing back to the sliding window:  
\begin{equation}
    \begin{split}
        &p_{i,f}(x_{k:0},s_{i},s_{j})=\\
        &=p_{f}(x_{k:n})\cdot p_{i,f}(s_{i},s_{j}|x_{k:n})
        \cdot \prod_{l=n}^{1}p_{i,f}(x_{l-1}|x_{m+l:l},s_{i},s_{j})\\
        &=p_{i,f}(x_{k:n},s_{i},s_{j})
        \cdot \prod_{l=n}^{1}p_{i,f}(x_{l-1}|x_{m+l:l},s_{i},s_{j})
    \end{split}
    \label{eq:fusedFactorizedAugReduced_3}
\end{equation}
We can now take natural logarithm and subtract eq. (\ref{eq:fusedFactorizedAugReduced_3}) from (\ref{eq:fusedFactorizedAugReduced_2}):
\begin{equation}
    \begin{split}
        &\log  p_{i,f}(s_{i},s_{j}|x_{k:n})=\log  p_{f}(s_{i},s_{j}|x_{k:0})\\
        &+\sum_{l=n}^{1}\bigg ( \log p_{i,f}(x_{l-1}|x_{m+l:l})-\log  p_{i,f}(x_{l-1}|x_{m+l:l},s_{i},s_{j}) \bigg )
    \end{split}
    \label{eq:fused_ownship}
\end{equation}
\od{Now it is left to come up with an algorithm to efficiently compute the distributions given in (\ref{eq:fused_ownship}) , (\ref{eq:ownship_Update}).}

\subsubsection{In Practice}
Assume:
\begin{enumerate}
    \item The assimilation process described in \ref{ssec:slidingWin} is efficient enough. 
    \item We don't need to communicate $p(x_{n-1:0}|x_{k:n})$ because it is equal between agents \textbf{(Maybe only true when $n-1$ is the last fusion step)}. \od{I'm not sure this is a good assumption}
\end{enumerate}
Adapting eq. (\ref{eq:logExactFusion_3states_B}) to AS:
\begin{equation}
    \begin{split}
        \log p_f(X_{k:0}) &= \log p_i(x_{k:0})+\log p_j(x_{k:0})-\log p_c(x_{k:0}) \\ &+\log p_i(s_i|x_{k:0})+\log p_j(s_j|x_{k:0})\\
        &=\log p_i(x_{k:0},s_i)+\log p_j(x_{k:n})\\
        &+\log p_j(x_{n-1:0}|x_{k:n})-\log p_c(x_{k:n})\\
        &-\log p_c(x_{n-1:0}|x_{k:n})+\log p_j(s_j|x_{k:0}),
    \end{split}
    \label{eq:slidingWinBDF}
\end{equation}
but from assumption 2 above $\log p_j(x_{n-1:0}|x_{k:n})=\log p_c(x_{n-1:0}|x_{k:n})$, so this can be written as
\begin{equation}
    \begin{split}
        \log p_{i,f}(X_{k:0}) &= \log p_i(x_{k:0},s_i)+\log p_j(x_{k:n})\\
        &-\log p_c(x_{k:n})+\log p_j(s_j|x_{k:0})
    \end{split}
     \label{eq:slidingWinBDF_i}
\end{equation}
this can be written also for the fusion at agent \emph{j}:
\begin{equation}
    \begin{split}
        \log p_{j,f}(X_{k:0}) &= \log p_j(x_{k:0},s_j)+\log p_i(x_{k:n})\\
        &-\log p_c(x_{k:n})+\log p_i(s_i|x_{k:0}).
    \end{split}
     \label{eq:slidingWinBDF_j}
\end{equation}
It is important to note that after fusion $p_{j,f}(X_{k:0})=p_{i,f}(X_{k:0})$, the two equations are different to reduce local computation complexity. \\

The next step is breaking the distribution back to the sliding window dimensions. Define $w$ to be the "slicing" window size, this will determine the maximum size of the matrix that we need to invert in the Gaussian case ($w\times n_x$, where $n_x$ is the number of states we need for conditional independence, which is 4 in our example). 
Starting from $p_f(X_{k:0})$:
\begin{equation}
    \begin{split}
        &p_f(X_{k:0})=p_f(x_{k:0},s_i,s_j)\\
        &=p_f(x_{k:w},s_i,s_j)\cdot p_f(x_{w-1:0}|x_{k:w},s_i,s_j)\\
        &=p_f(x_{k:2w},s_i,s_j)\cdot p_f(x_{2w-1:w}|x_{k:2w},s_i,s_j)\\
        &\cdot p_f(x_{w-1:0}|x_{k:w},s_i,s_j)\\
        &=p_f(x_{k:n},s_i,s_j)\cdot \prod^{n/w}_{l=1}
        p_f(x_{l\cdot w-1:(l-1)\cdot w}|x_{k:l\cdot w} ,s_i,s_j).
    \end{split}
\end{equation}
This equation can be translated into a recursive algorithm to compute and store the $n/w$ distributions, $p_f(x_{l\cdot w-1:(l-1)\cdot w}|x_{k:l\cdot w} ,s_i,s_j)$, and the sliding window distribution $p_f(x_{k:n},s_i,s_j)$.
